# Supplementary material for: Commonsense mining as knowledge base completion? A study on the impact of novelty
Source: arXiv:1804.09259 source file (2018-04-24)
Supplement: Supplementary file 1 [file appendix.tex]

\documentclass[11pt,a4paper]{article}
\usepackage[hyperref]{naaclhlt2018}
\usepackage{times}
\usepackage{latexsym}

\usepackage[english]{babel}
\usepackage[utf8]{inputenc}
\usepackage[T1]{fontenc}
\usepackage{amsfonts} 
\usepackage{booktabs}
\usepackage{setspace}
\usepackage{subcaption}
\usepackage{graphicx}

\title{Appendix}
\begin{document}

\appendix{Test}

\end{document}
